# Supplementary material for: Observation of Quantized Klein Tunneling in a Dielectric Resonator Chain
Source: arXiv:2403.02047 source file (2024-06-29)
Supplement: Supplementary file 1 [file SM.pdf]

# Supplemental Material for

# Observation of Quantized Klein Tunneling in a Dielectric Resonator Chain

Rui-Jie Zhang,[1,*] Xiao-Zhen Peng,[1,*] Ri-Zhen Yang,[1] Rui-Hua Ni,[1] Yong-Yin Hu,[1] Hong-Ya Xu,[1,†] and Liang Huang[1,‡]

[1]*Lanzhou Center for Theoretical Physics, Key Laboratory of Theoretical Physics of Gansu Province,*
*Key Laboratory of Quantum Theory and Applications of MoE,*
*and School of Physical Science and Technology, Lanzhou University, Lanzhou, Gansu 730000, China*

(Dated: June 13, 2024)

**CONTENTS**

I. Further details of the experimental setup 1

II. Extracting the parameters 3

III. Further details of the LDOS data 6

References 7

## I. FURTHER DETAILS OF THE EXPERIMENTAL SETUP

The settings of the experiment is shown in Fig. S1. The cylindrical dielectric resonators with a high permittivity $\varepsilon = 37$ and height 5 mm (Ether, BT37 series) are firstly placed in the feeding grooves. For each resonator, the high precision automatic robotic arm catches the resonator via an air sucker, moves it to the upper right groove, and lets it fall freely to reach a position that depends solely on its diameter. This process calibrates the initial position of the resonators and is labeled by ① in Fig. S1(a). Then the automatic robotic arm moves to a prescribed position on top of the resonator in this groove, and takes it to the copper plate with a programmed position, as labeled by ②. This process repeats automatically to form the dimer chain (see the Supplemental Video for a complete cycle of placing the resonators). The feeding grooves can contain up to 90 resonators at a time, that can be placed on the copper plate according to programmed coordinates. The lower inset of Fig. S1(a) shows the schematics and parameters of the groove, leading to a $\Delta y = 0.35$ mm negative shift for the 3.93 mm resonators, which needs to be compensated when placing them. The loop antenna [upper inset of Fig. S1(a)] is fixed on the top plate, which is supported and can move along on the slide-rail. The alignment of the dimer chain placed by the automatic robotic arm (the calibration of its coordinate system) and the loop antenna moving along the slide-rail has been calibrated based on a laser level.

We have in total 225 resonators of 4 mm radius. We measure their resonances of the S-mode in the frequency range 6.5-7 GHz with a kink antenna, and choose 30 resonators whose resonant frequencies are most close to each other for our experiments. For the 3.93 mm resonators, we choose 30 from in total of 115 resonators. The frequency responses of the reflection spectra of these 60 resonators are plotted in Fig. S2(a). For an isolated resonance, the reflection spectrum $S_{11}$ follows [1]

$$1 - |S_{11}(f)|^2 \simeq \frac{2\sigma\Gamma}{(f-\nu_0)^2 + \Gamma^2} |\psi(x)|^2 \tag{S1}$$

where $f$ is the scanning frequency, $\nu_0$ is the bare resonant frequency for the resonator, $\sigma$ is the antenna coupling strength and is nearly a constant, $\Gamma$ is the spectral width due to Ohmic loss in the top and bottom metallic plates. The fitting to this formula

* these authors contributed equally to this work.
† Corresponding author: xuhongya@lzu.edu.cn
‡ Corresponding author: huangl@lzu.edu.cn

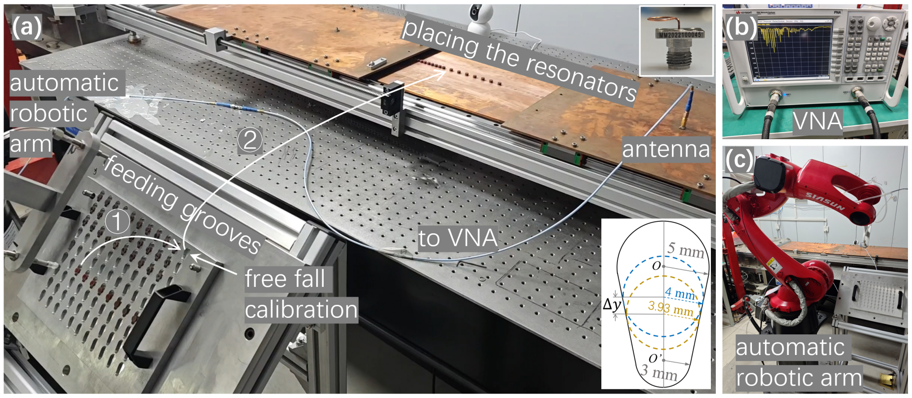


FIG. S1. The experimental settings. (a) The dielectric resonator in the feeding grooves is moved by the automatic robotic arm sequentially to the upper right groove, let it fall freely to reach a steady position depends solely on its diameter, as labeled by ①, which calibrates the initial position of the resonators. Then the automatic robotic arm repositions to a prescribed location above the resonator in this groove, and places it on the copper plate to form the dimer chain, as labeled by ②. The loop antenna (upper inset) is fixed on the top plate, which is supported and can move along on the slide-rail. Lower inset: schematics and parameters of the groove, leading to a $\Delta y = 0.35$ mm downward shift for the 3.93 mm resonators, which needs to be compensated when placing them. (b) The vector network analyser (Agilent N5227A). (c) The automatic robotic arm (Siasun, T12B-14, ±0.03 mm).

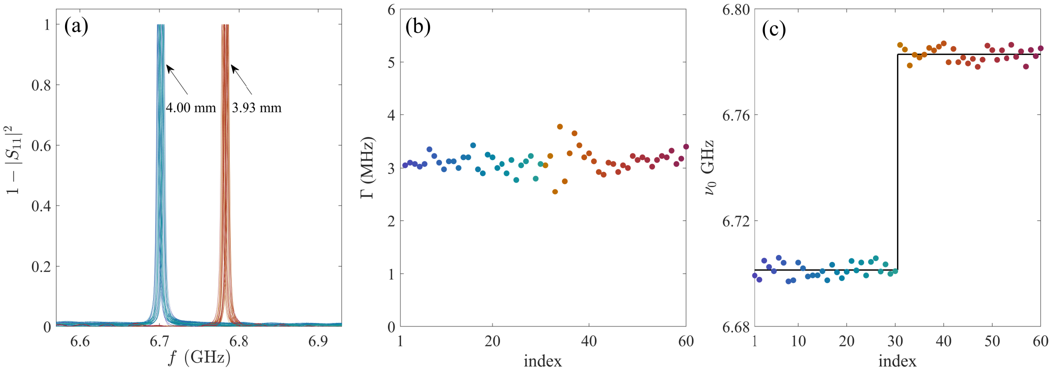


FIG. S2. (a) The frequency responses of the 30 $r = 4$ mm resonators and the 30 $r = 3.93$ mm resonators used in our experiments. (b) The peak width $\Gamma$ for the resonators with index 1-30 for the 4 mm resonators, and 31-60 for the 3.93 mm resonators. (c) The resonant frequencies $\nu_0$ of these resonators. The line indicates the mean value of each group.

yields the bare resonant frequency $\nu_0$ and the width $\Gamma$, which are shown in Fig. S2(b) and Fig. S2(c,d). The mean bare resonant frequencies are 6.7014 GHz for the 4 mm resonators, and 6.7829 GHz for 3.93 mm resonators. The resonant frequencies show good clustering for each case, and the width $\Gamma$ is about 3 MHz. The resonant frequencies $\nu_0$ of these resonators show a good step profile.

The resonators are then placed on the bottom copper plate in the form described in the main text, and the reflection spectra is measured as $S_{11}^{(0)}(x, f)$ by positioning the loop antenna (fixed on the top copper plate) on top of each resonator. To remove the effect solely due to the cavity, we have measured the reflection spectrum $S_{11}^{(e)}$ for the empty cavity when no resonators are placed. As the cavity is much larger than the spatial scale of the dimer chain, for the positions of the resonators in the dimer chain, $S_{11}^{(e)}$ is almost the same. Thus $S_{11}(x, f) = S_{11}^{(0)}(x, f) - S_{11}^{(e)}(f)$ is the reflection spectra due to the resonators, which will be used for further analysis. An example of the absolute value, the argument, the real part, and the imaginary part of the reflection spectra for the 25th resonator of Experiment 1 is plotted in Fig. S3.

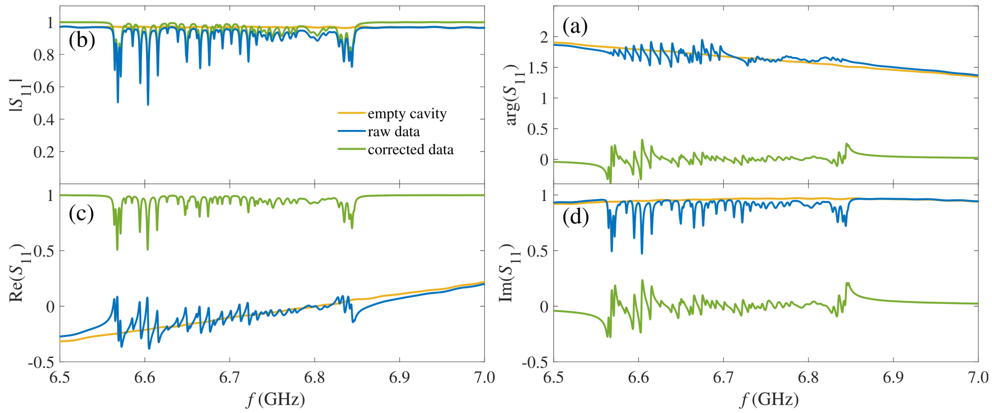


FIG. S3. The blue curves are the measured reflection spectrum $S_{11}^{(0)}$ from the 25th resonator of the dimer chain for Experiment 1, the yellow curves are the measured $S_{11}^{(e)}$ for the empty cavity. The corrected reflection spectra $S_{11} = S_{11}^{(0)} - S_{11}^{(e)}$ are the green curves, which will be used for further analysis. (a-d) are for the absolute value, the argument, the real part, and the imaginary part, respectively.

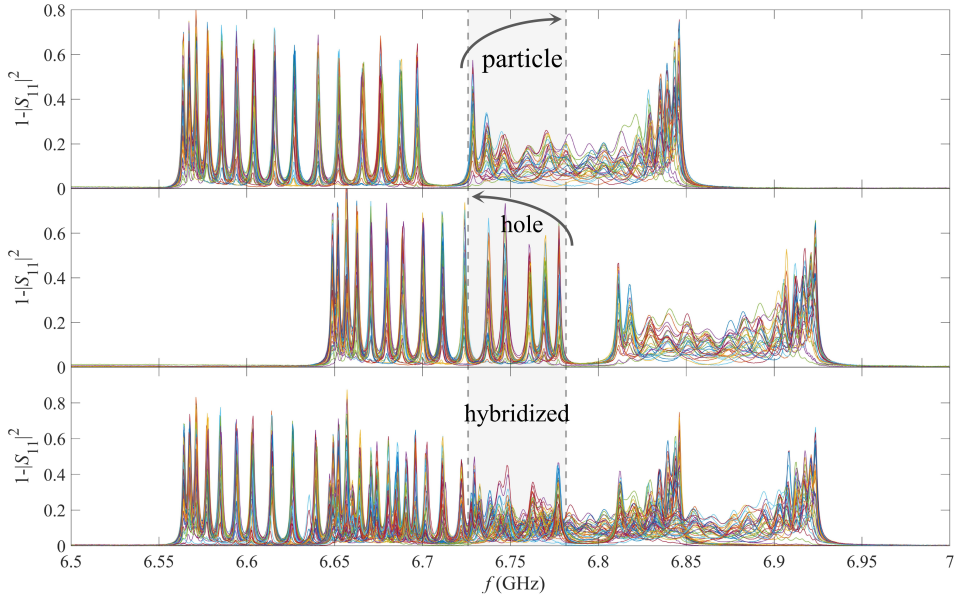


FIG. S4. (a) The reflection spectra measured on top of each resonator for the dimer chain of the 30 $r = 4$ mm resonators alone. (b) The reflection spectra for the dimer chain of the 30 $r = 3.93$ mm resonators alone. (c) The reflection spectra for the dimer chain simulating the Dirac system with a step potential, i.e., the 30 $r = 4$ mm resonators on the left, and the 30 $r = 3.93$ mm resonators on the right. The shaded region bounded by the dashed vertical lines indicates the Klein tunneling regime. The indices of the resonators are 1, 2, 3, $\cdots$, 58, 59, 60. This is denoted as Experiment 1 (E1).

## II. EXTRACTING THE PARAMETERS

We have carried out a series of four experiments: E1) $(N_L, N_R) = (15, 15)$; E2) the same as E1 but with an independent placement of the resonators whose order is the same as E1 and an independent measurement; E3) $(N_L, N_R) = (15, 15)$ but with a random permutation for both the resonators on the left side and those on the right side, respectively; E4) $(N_L, N_R) = (15, 9)$. To be convenient for the following analysis, here, similar to Fig. 2 in the main text showing the data for Experiment 1, we plot in Figure S4 the reflection spectra measured on top of each resonator for Experiment 1.

For each experiment, besides the measurement for the whole system [Fig. S4(c)], i.e., 4 mm dimer chain on the left and 3.93 mm dimer chain on the right, we need to measure the reflection spectra for the 4 mm dimer chain alone to determine the

parameters $mc^2$, $c\hbar$, and $f_0$ for the particle states [above the band gap, Fig. S4(a)], and that for the 3.93 mm dimer chain alone to determine the parameters $mc^2$, $c\hbar$, and $f_0$ for the hole states [below the band gap, Fig. S4(b)].

For the particle states, when keeping only the nearest neighbor couplings ($v$,$w$) and neglecting the next-nearest neighbor coupling $t$, the dispersion relation for the particle states above the gap of the Su-Schrieffer-Heeger (SSH) model is [2]

$$(f-f_0)^2 =(v+w\cos k'a_0)^2+(w\sin k'a_0)^2, \tag{S2}$$
$$\simeq(v-w)^2+(-w)^2k^2a_0^2,$$
$$=m^2c^4+c^2\hbar^2k^2, \tag{S3}$$

where $f_0$ is the frequency of the Dirac point (corresponding to $E=0$), $k'$ is the wavevector, $k=k'-(-\pi/a_0)$. Note that a small next-nearest neighbor coupling only shifts $f_0$ [2], but does not change the values of $v$ and $w$ (or $mc^2$ and $c\hbar$). Thus the fitting with Eqs. (S2) or (S3) will take into account of the effect of the next-nearest neighbor coupling directly into the value of $f_0$.

Conventionally, from Eq. (S2), the parameters $v$ and $w$ can be fitted from the high symmetric points at $k'=0$ and $k'=\pi/a_0$, then to yield $mc^2=v-w$, $c\hbar=wa_0$. However, for our case, since our goal is to simulate the Dirac system with Klein tunneling, we shall mainly focus on the region of the SSH system around the band gap, thus it would be better to directly fit with Eq. (S3) for the parameters $mc^2$, $c\hbar$ and $f_0$ using the data of the resonances $(f_n,k_n)$ close to the band gap. For this reason, we would need the calculation of the local density of states (LDOS), the density of states (DOS), the resonant frequencies, and the wavefunction intensities from the reflection spectra for the 4 mm dimer chain alone for the particle states, and also that for the 3.93 mm dimer chain alone for the hole states.

In particular, following the standard procedure in Ref. [1], the LDOS can be derived through the $g$ function,

$$g(x,f)=\frac{|S_{11}(x,f)|^2}{\langle|S_{11}(x,f)|^2\rangle_f}\varphi'_{11}(x,f)$$
$$=\frac{|S_{11}(f)|^2}{\langle|S_{11}|^2\rangle_f}\frac{\mathrm{Im}(S'_{11})\,\mathrm{Re}(S_{11})-\mathrm{Im}(S_{11})\,\mathrm{Re}(S'_{11})}{|S_{11}|^2}, \tag{S4}$$

where $\varphi_{11}(x,f)=\mathrm{Arg}[S_{11}(x,f)]$, " $'$ " is the derivative with respect to the scanning frequency $f$, and $\langle\cdot\rangle_f$ is the average over frequency $f$. With the argument, the real part, and the imaginary part of $S_{11}$, the corresponding $g$ function can be calculated. For isolated resonance, with Eq. (S1), the $g$ function can be further written as [1]

$$g(x,f)\simeq-\frac{\sigma}{\Gamma\langle|S_{11}(x,f)|^2\rangle_f}\sum_n|\psi_n(x)|^2\delta(f-f_n)$$
$$\simeq-\frac{\sigma}{\Gamma\langle|S_{11}(x,f)|^2\rangle_f}\rho(x,f). \tag{S5}$$

Thus $g(x,f)$ approximates the LDOS $\rho(x,f)$, and the wavefunction intensity $|\psi_n(x)|^2$ can be approximated by taking $\max_{f\approx f_0}[g(x,f)]$.

The DOS can be approximated by the average of the $g$ function over all positions $x$, i.e., $\mathrm{DOS}(f)\sim\langle g(x,f)\rangle_x$. In general, the DOS $\rho(f)=\int\rho(x,f)\mathrm{d}x=\sum_n\delta(f-f_n)\simeq\sum_n\frac{1}{\pi}\frac{\Gamma_n}{\Gamma_n^2+(f-f_n)^2}$. Thus for frequencies around an isolated peak $f_n$,

$$\rho(f)\propto\frac{\Gamma_n}{\Gamma_n^2+(f-f_n)^2}. \tag{S6}$$

Experimentally, for isolated DOS peaks, the fitting to the Lorentzian line shape Eq. (S6) yields the resonant frequency $f_n$ and the width $\Gamma_n$.

For the reflection spectra of the 4 mm dimer chain (with 15 dimers) alone, as shown in Fig. S4(a), the first 5 resonances above the band gap are exploited to extract the resonant frequencies $f_n$ and the corresponding wavevectors $k_n$, as follows. From the $S_{11}$s in Fig. S4(a) measured from each resonator, the LDOS and the DOS are obtained for the dimer chain. Since the chain has only 15 dimers (30 resonators), the peaks are well separated. The resonant frequencies $f_n$ are determined by fitting the peaks of DOS to Eq. (S6). For each $f_n$, the corresponding LDOS or the wavefunction intensities $|\psi_n(x)|^2$ can be obtained. Then for the $A$ sublattices, Fourier transformation for $|\psi_n^{(A)}(x)|^2$, i.e., $C_n^{(A)}(k)=\int e^{\mathrm{i}kx}|\psi_n^{(A)}(x)|^2\mathrm{d}x\simeq\sum_{j=1}^{15}e^{\mathrm{i}kx_j}|\psi_n^{(A)}(x_j)|^2a_0$ with

TABLE I. The extracted resonant frequencies $f_n$ and the corresponding wavevectors $k_n$ for the data in Fig. S4(a).

| | $n=1$ | $n=2$ | $n=3$ | $n=4$ | $n=5$ |
|---|---|---|---|---|---|
| $f_n$ (GHz) | 6.729 | 6.737 | 6.746 | 6.760 | 6.771 |
| $k_n^{(A)}a_0$ | 0.1950 | 0.3129 | 0.5378 | 0.7123 | 0.9340 |
| $k_n^{(B)}a_0$ | 0.1918 | 0.3255 | 0.5393 | 0.7186 | 0.9481 |
| $k_n a_0$ | 0.1934 | 0.3192 | 0.5385 | 0.7154 | 0.9411 |

a fine enough step for $k$ is carried out, where $x_j$ is the position for the $A$ site of the $j$th dimer. This yields the dominant peak of $C_n^{(A)}(k)$ at $\widetilde{k}_{x,n}^{(A)}$, half of which gives the corresponding wavevector $k_n^{(A)} = \widetilde{k}_{x,n}^{(A)}/2$. The wavevector $k_n^{(B)}$ for $B$ sublattices can be obtained similarly. The results of $f_n$, $k_n^{(A)}$ and $k_n^{(B)}$ for the data in Fig. S4(a) are listed in Table I. The average of $k_n^{(A)}$ and $k_n^{(B)}$ will be used for the corresponding wavevectors $k_n$.

For each set of $f_n$ and $k_n$ for the 4 mm dimer chain (all with 15 dimers), one could then fit with Eq. (S3) to yield $f_0$, $mc^2$ and $c\hbar$ simultaneously for the particle states. The fitting results of the four sets of data are listed in Table II.

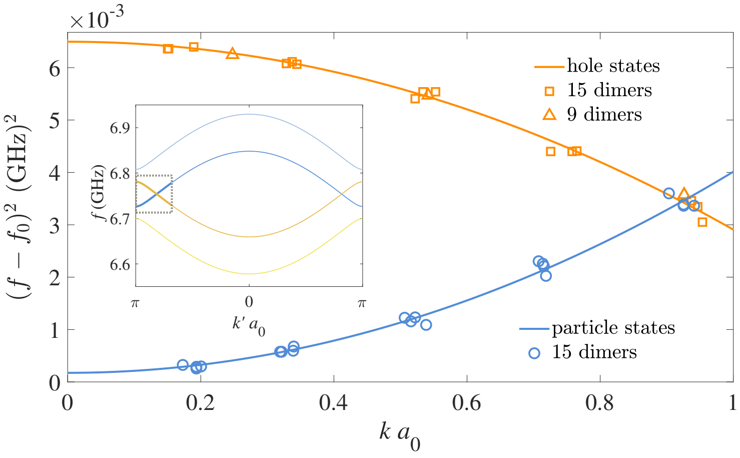


FIG. S5. The data points are the extracted $f_n$ and $k_n$ for both particle states (blue) and hole states (yellow), and the curves are Eqs. (S3) and (S7) with the fitted parameters of $mc^2 = 12.894$ MHz, $c\hbar/a_0 = 61.325$ MHz, $f_0 = 6.7130$ GHz for 4 mm dimer chain, and $f_0 = 6.7945$ GHz for 3.93 mm dimer chain, corresponding to $\Delta f = 81.5$ MHz. Inset shows the dispersion relation where the lower set is for the 4 mm dimer chain, and the upper set is for the 3.93 mm dimer chain, the dashed rectangle indicates the range of the main panel including the particle states for the 4 mm case and the hole states for the 3.93 mm case.

On the other hand, the resonant frequencies $f_n$ and the corresponding wavevectors $k_n$ for the hole states (below the gap) from the reflection spectra for the 3.93 mm dimer chain, e.g., in Fig. S4(b), can also be obtained. Five resonances are used for the

TABLE II. The fitting results for the particle states of the 4 mm dimer chain with Eq. (S3) and the hole states of the 3.93 mm dimer chain with Eq. (S7).

| Data set | $mc^2$ (MHz) | $c\hbar/a_0$ (MHz) | $f_0$ (GHz) |
|---|---|---|---|
| 4 mm, E1 | 12.1526 | 60.8122 | 6.71300 |
| 4 mm, E2 | 13.3601 | 61.8882 | 6.71301 |
| 4 mm, E3 | 12.8918 | 63.5743 | 6.71303 |
| 4 mm, E4 | 13.7102 | 61.8333 | 6.71302 |
| 3.93 mm, E1 | 12.8302 | 59.5952 | 6.79451 |
| 3.93 mm, E2 | 13.5009 | 59.2377 | 6.79452 |
| 3.93 mm, E3 | 12.0759 | 59.4066 | 6.79452 |
| 3.93 mm, E4 | 11.3398 | 59.6743 | 6.79452 |

case of 15 dimers (three experiments, E1-E3), and four peaks are used for the case of 9 dimers (one experiment, E4). For the 4 sets of $f_n$ and $k_n$ of the 3.93 mm dimer chains, a similar approach to fitting with

$$(f - f_0)^2 = m^2c^4 - \hbar^2 c^2 k^2 \tag{S7}$$

yields $f_0$, $mc^2$ and $c\hbar$ for the hole states. The fitted values are also listed in Table II. Averaging both the results for particle states and hole states leads to $mc^2 = 12.894$ MHz, $c\hbar/a_0 = 61.325$ MHz, and $f_0 = 6.713$ GHz, $\Delta f = 81.5$ MHz, which will be used in the theory in the main text. The extracted data points of $f_n$ and $k_n$ for both the particle states and the hole states are plotted in Fig. S5, together with the dispersion relations Eqs. (S3) and (S7) with the above fitting parameters. One can see that the data points follow the fitting curves well.

## III. FURTHER DETAILS OF THE LDOS DATA

From the reflection spectra of the whole system, e.g., those for E1 in Fig. S4(c), one can obtain the LDOS via the $g$ function [Eq. (S4)], from which the DOS and the wavefunction intensities can be obtained (see Eqs. (S5) and (S6) and discussions there).

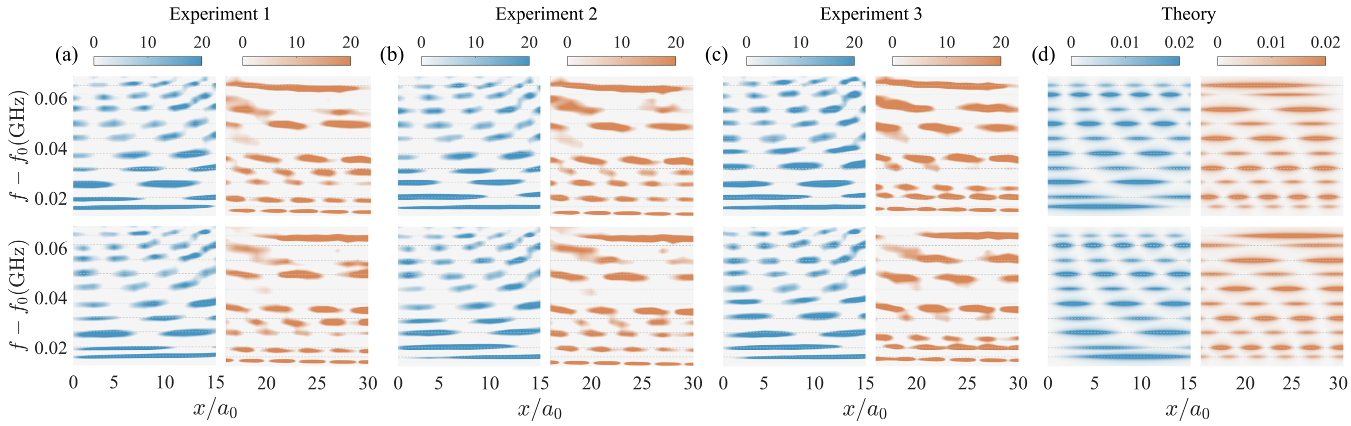


FIG. S6. The LDOS for the (15, 15) case in the regime of Klein tunneling. Upper (lower) parts are the LDOS for $A$ ($B$) sublattices or the first (second) component. (a-c) are for the three experiments E1-E3, respectively. The dashed horizontal lines indicate the eigenlevels from the theory. (d) is the theoretically obtained LDOS [Eq. (S8)] with an artificial fixed resonance width $\Gamma_n = 0.0009$ to be comparable with the experimental results. The vertical axis is $E = f - f_0$. Blue (orange) on the left (right) side for each panel indicates the intensities for particles (holes).

Theoretically, with the obtained eigenlevels $E_n$ and eigenwavefunctions $\psi_n(x)$, the LDOS can be written as

$$\begin{aligned}\rho(x, E) &= \sum_n |\psi_n(x)|^2 \delta(E - E_n) \\ &\simeq \sum_n |\psi_n(x)|^2 \frac{1}{\pi} \frac{\Gamma_n}{\Gamma_n^2 + (E - E_n)^2},\end{aligned} \tag{S8}$$

where $\Gamma_n$ is the artificial resonance width in order to compare with the experimental results.

Figure S6 plots the obtained 3 sets of LDOS for different experiments together with the theoretically obtained LDOS, for the $(N_L, N_R) = (15, 15)$ case in the Klein tunneling regime. Although there are perceptible difference in the details of the three experimental data, they share clearly common features of the LDOS patterns.

Figure S7 compares the experimental data and the theory for the LDOS for the (15, 9) case. Again, the experimental resonances agree with the predicted eigenlevels, and the LDOS patterns share common features regarding the variation of the number of peaks vs the energy (frequency), and the boundary conditions for the two components.

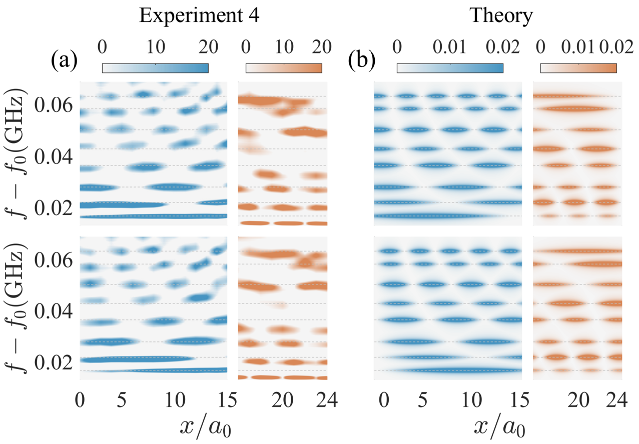


FIG. S7. The LDOS for the (15, 9) case. Upper (lower) parts are the LDOS for $A$ ($B$) sublattices or the first (second) component. (a) is for the experimental data E4, (b) is the theory with $\Gamma_n = 0.0009$, and the vertical axis is $E = f - f_0$.

Importantly, Figs. S6 and S7 show concretely that the observed Klein tunneling states are quantized and are insensitive to different realizations. They agree with the theoretical predications well.


[1] Matthieu Bellec, Ulrich Kuhl, Gilles Montambaux, and Fabrice Mortessagne. Tight-binding couplings in microwave artificial graphene. *Phys. Rev. B*, 88:115437, Sep 2013.

[2] J. Asbóth, László Oroszlány, and András Pályi. *A Short Course on Topological Insulators*. Springer Cham, 01 2016.
